# Supplementary material for: Collaboration with Cellular Networks for RFI Cancellation at Radio Telescope
Source: arXiv:2210.17083 source file (2022-10-31)
Supplement: Supplementary file 1 [file additional.tex]

\section{Additional Results}

\begin{comment}

\begin{figure*}[h]
\centering
\includegraphics[width=1\linewidth]{figs/uplink_block_rfi_updated.png}
\caption{Sample Uplink Scenrario}
    \label{fig:uplink_block}
    \vspace{-0pt}
\end{figure*}

\begin{figure*}[h]
\centering
\includegraphics[width=0.56\linewidth]{figs/illustration_UL_DL_channel.png}
\caption{RFI propagation from LTE cell: Uplink and Downlink}
    \label{fig:uplink_block_close}
    \vspace{-0pt}
\end{figure*}

\end{comment}

\begin{comment}
\begin{figure*}[h]
\centering
\begin{subfigure}[b]{0.4\linewidth}
    \includegraphics[width=\linewidth]{figs/macroCell_rqf.png}
    \caption{Urban Macro-cell}
    %\caption{\note{PSD of astro signal}\\\greg{use xlim() on all plots}}
    \label{fig:astro}
\end{subfigure}
\begin{subfigure}[b]{0.4\linewidth}
    \includegraphics[width=\linewidth]{figs/microCell_rqf.png}
    \caption{Urban Micro-cell}
    \label{fig:lte_psd}
\end{subfigure}
\begin{subfigure}[b]{0.4\linewidth}
    \includegraphics[width=\linewidth]{figs/ruralMacro_rqf.png}
    \caption{Rural Macro-cell} %\greg{get rid of this one?}}
    \label{fig:signals_time_domain}
\end{subfigure}
\begin{subfigure}[b]{0.4\linewidth}
    \includegraphics[width=\linewidth]{figs/suburbMacro_rqf.png}
    \caption{Suburban Macro-cell}
    \label{fig:composite_psd}
\end{subfigure}
\begin{subfigure}[b]{0.4\linewidth}
    \includegraphics[width=\linewidth]{figs/in2outdoor_rqf.png}
    \caption{Indoor to Outdoor Urban Channel}
    \label{fig:composite_psd}
\end{subfigure}
\caption{Reconstruction Quality in presence of RFI from Uplink Signal - Different Channel scenarios}
%I am guessing this has been resolved ---- \greg{(a) and (b) don't have the same bandwidth, so (c) is confusing because the time indexes are not aligned for the three signals. Could we overlap the filtered/decimated LTE spectrum on top of (b)?}}
\label{fig:uplink_rqf}
\vspace{-15pt}
\end{figure*}

\end{comment}
